# Supplementary material for: PartCo: Part-Level Correspondence Priors Enhance Category Discovery
Source: arXiv:2509.22769 source file (2026-05-21)
Supplement: Supplementary file 1 [file impacts.tex]

\section{Impact Statement}
\label{supp:impacts}
The development of the Part-Level Correspondence Prior (PartCo) framework represents a significant advancement in category discovery, especially in recognizing fine-grained categories and enabling more robust intelligent systems in real-world scenarios. Fine-grained category recognition is essential in fields such as biodiversity conservation, where precise species identification supports ecological monitoring, and in healthcare, where detailed analysis of medical images could potentially lead to improved disease diagnosis and personalized treatment plans. However, the deployment of PartCo also presents potential ethical and societal challenges. Enhanced image recognition capabilities could be misused in surveillance systems, raising significant privacy concerns. There is a risk that biased training data may lead to unfair or discriminatory outcomes. To mitigate these risks, it is essential to implement robust data governance frameworks that ensure diversity and representativeness in training datasets, thereby minimizing biases. Privacy-preserving techniques and strict regulatory compliance should be prioritized to protect individual rights and prevent misuse in categorization tasks.
